# Supplementary material for: Discovering Language-neutral Sub-networks in Multilingual Language Models
Source: arXiv:2205.12672 source file (2022-10-30)
Supplement: Supplementary file 2 [file 8.appendix_sparsity_overlap.tex]

In Figure~\ref{fig:sparsity_overlap}, we compare the similarity between sparsity patterns found for each language across different layers of mBERT.
The pattern similarity is computed as the relative overlap ratio between masks~(i.e., $m_i$, $m_j$) from two sub-networks~(i.e, $\frac{m_i \cap m_j}{m_i \cup m_j}$).
To avoid crowding the plots, we only kept the language pairs that includes English.
The overlap trend for other pairs of languages is the same.

For the NER and XNLI tasks, the sparsity overlap increases as it goes deeper into layers, suggesting that top layers are more task-specific than the bottom layers for these two tasks.
This observation is related to findings of recent work from~\cite{merchant2020whathappens} and \cite{muller2021firstalign}, showing that fine-tuning impacts mainly the upper layers of the model and preserves the linguistic features learned during pre-training.
Here we do not compare the fine-tuned networks, but the best sub-networks for a task with their original pre-training initialization.
It means that, even without fine-tuning the networks, top layers contain more information useful for NLI and NER tasks.

For the MLM task, the pattern overlap is less than the two other increases up to middle layers, and then decreases afterwards.
As to the reason why the overlap goes down in the last few layers, one possible explanation is that
since the sub-networks was found for MLM, it might need more language-specific information to correctly predict the missing word.

\begin{figure*}

    \centering
    \subfloat{
        {\includegraphics[width=1\textwidth]{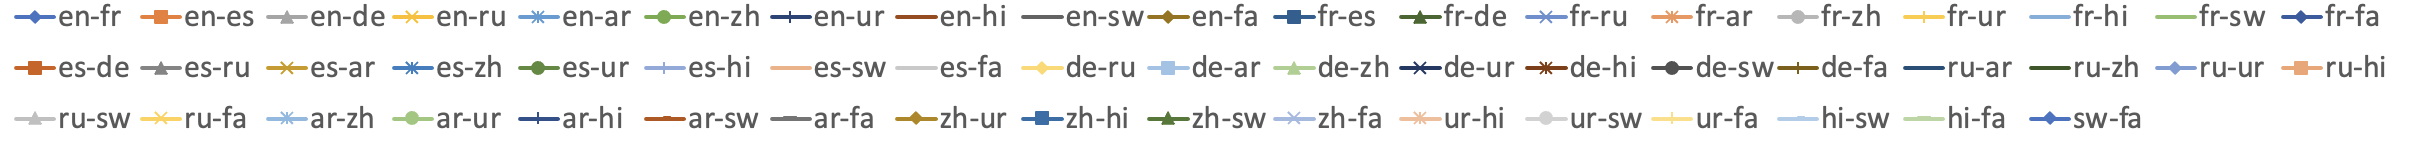}}
    }
    
    \addtocounter{subfigure}{-1}
    
    \centering
    \subfloat[MLM]{
        \label{fig:mlm_sparsity_overlap}
        {\includegraphics[width=0.32\textwidth]{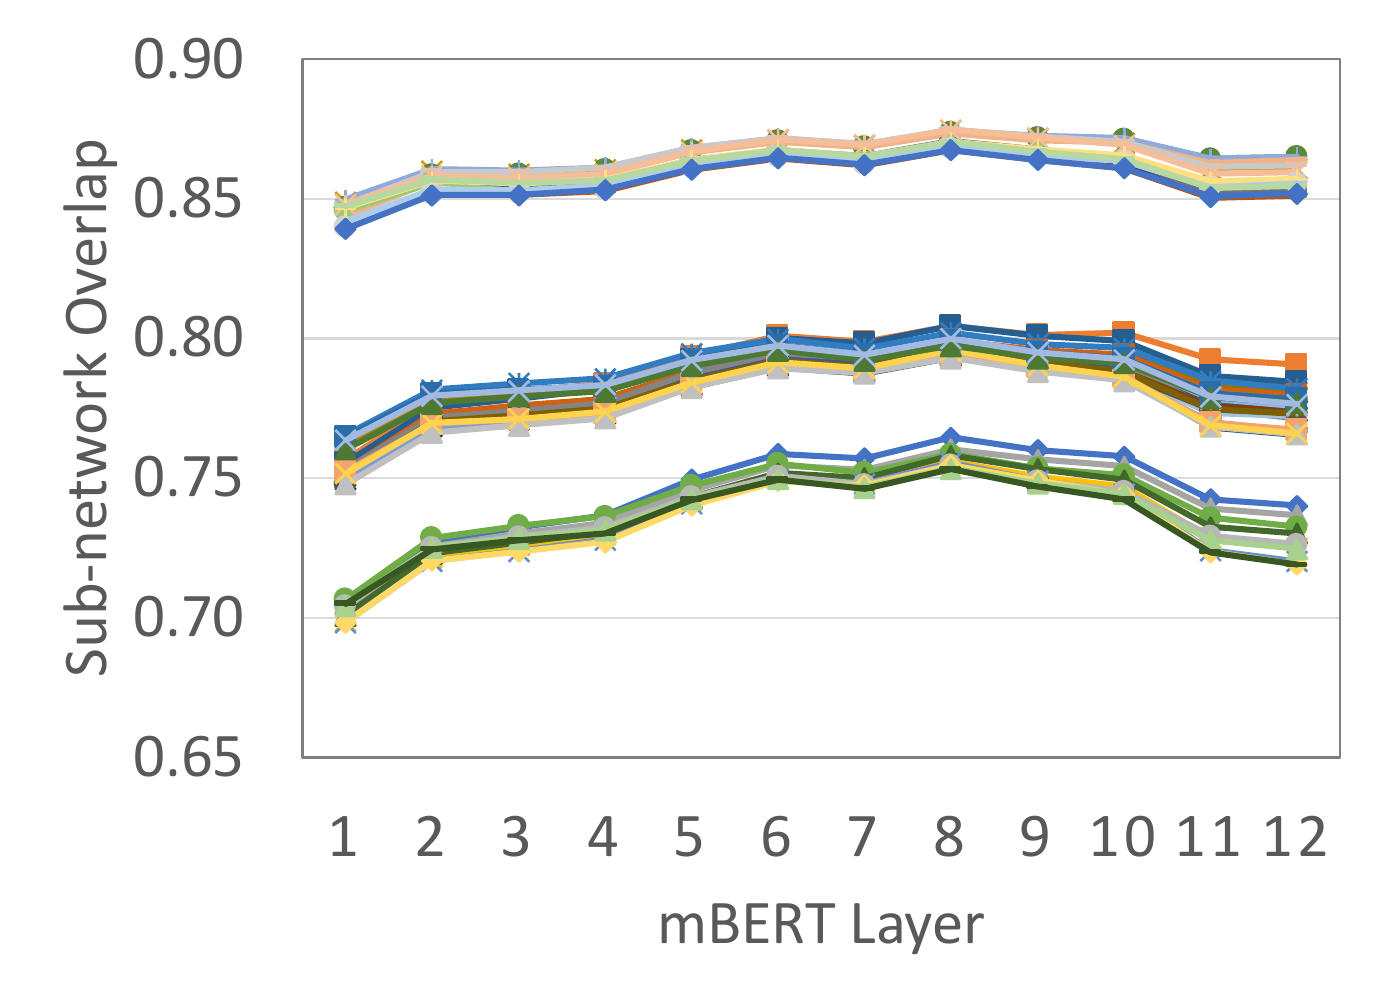}}
    }
    \centering
    \subfloat[NER]{
        \label{fig:ner_sparsity_overlap}
        {\includegraphics[width=0.32\textwidth]{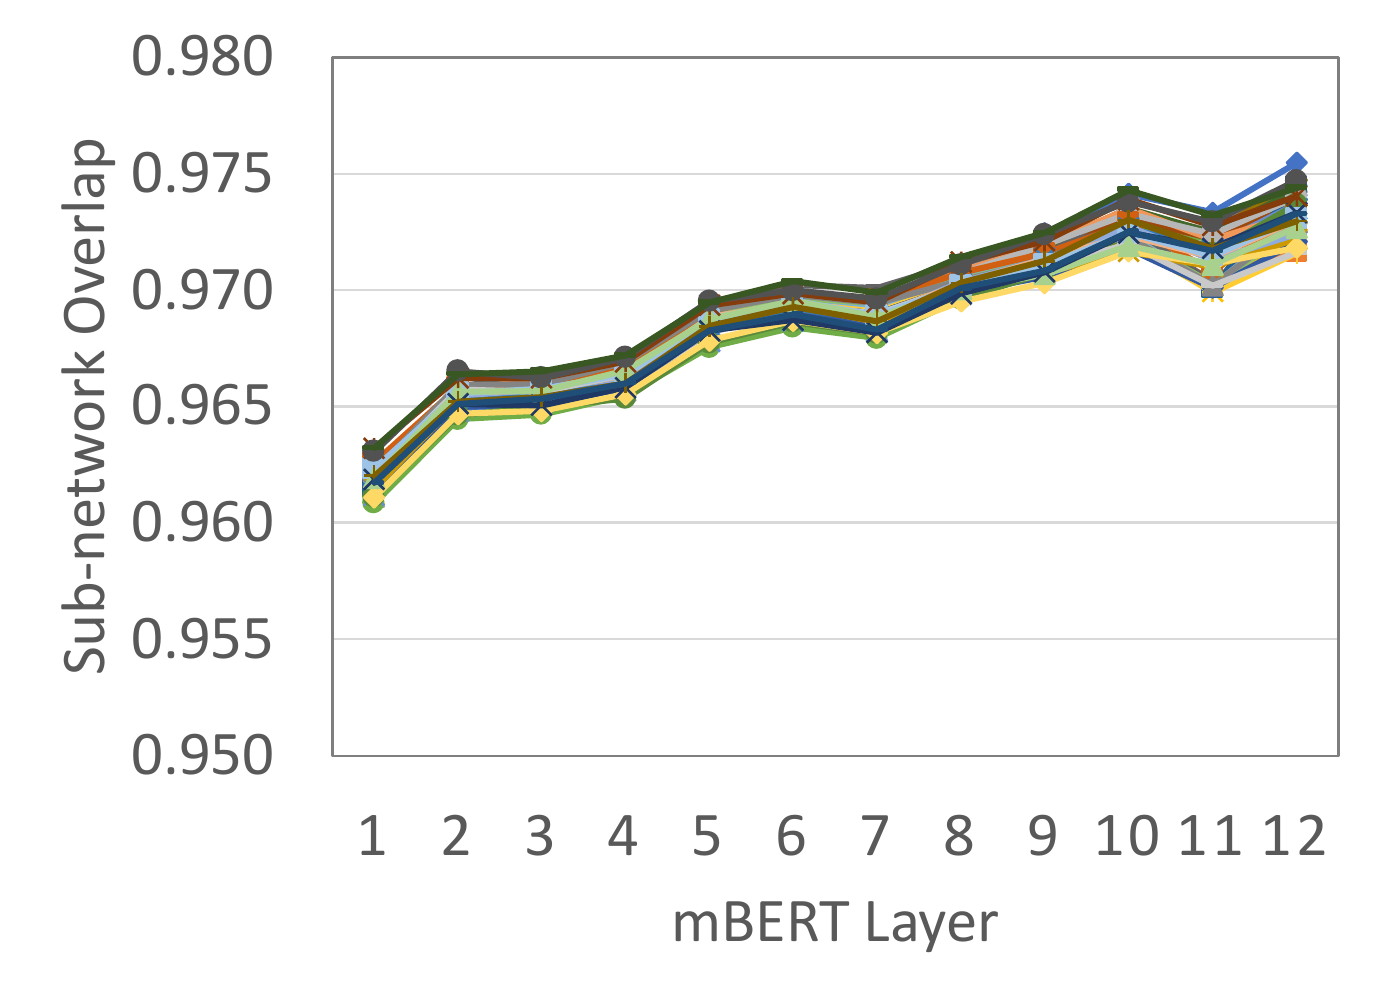}}
    }
    \centering
    \subfloat[XNLI]{
        \label{fig:xnli_sparsity_overlap}
        {\includegraphics[width=0.32\textwidth]{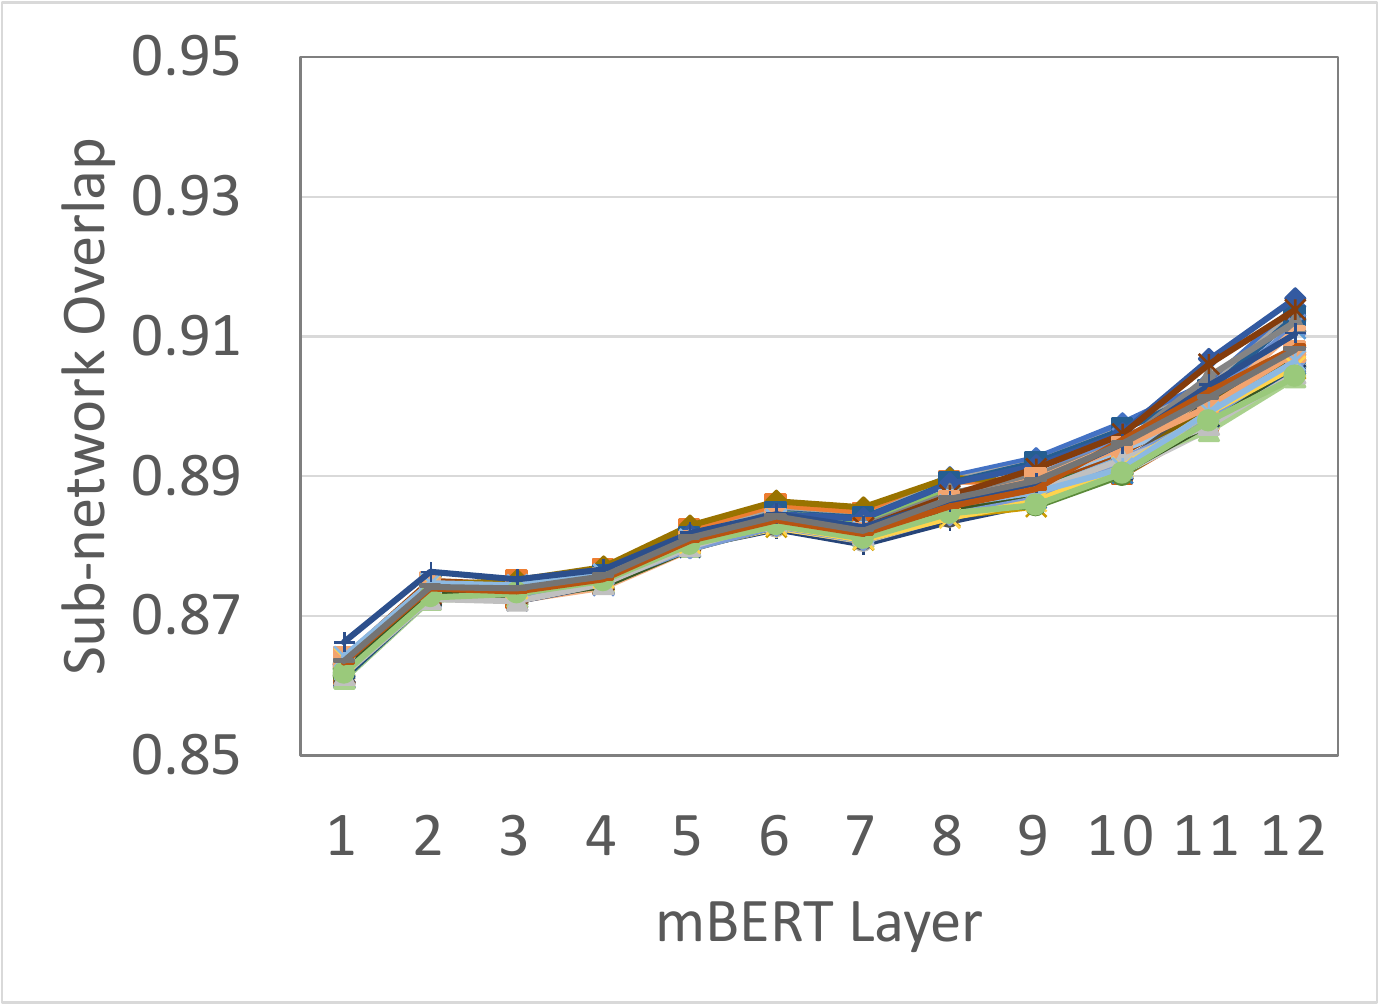}}
    }
    \caption{Sparsity pattern overlap between pruned sub-networks across different layers at 50\% sparsity level.}
    \label{fig:sparsity_overlap}
    \vspace{-4mm}
\end{figure*}
