# Supplementary material for: Discovering Language-neutral Sub-networks in Multilingual Language Models
Source: arXiv:2205.12672 source file (2022-10-30)
Supplement: Supplementary file 8 [file margine_based_scoring.tex]

\section{Margin-based Scoring}
\label{sec:scoring_func}
For the parallel sentence retrieval task, we use the scoring function from~\cite{artext2019margin}:
\begin{multline*}
s(x, y) = \frac{cos(x, y)}{\sum\limits_{z \in \mathcal{N}_{k}(x)} \frac{cos(x, z)}{2k} + \sum\limits_{z \in \mathcal{N}_{k}(y)} \frac{cos(y, z)}{2k}}
\end{multline*}

\noindent where $x$ and $y$ are two sentence representations and $\mathcal{N}_k(x)$ denotes the $k$ nearest neighbors of $x$ in the other language. 
We use $\mbox{margin}(a, b) = a/b$ as our margin function.
% \begin{multline*}
% \mbox{score}(x, y) = \mbox{margin}(cos(x, y), \\ \sum_{z \in NN_{k}(x)} \frac{cos(x, z)}{2k} + \sum_{z \in NN_{k}(y)} \frac{cos(y, z)}{2k})
% \end{multline*}

% \noindent where $x$ and $y$ are the two sentence representations and $NN_k(x)$ denotes the $k$ nearest neighbors of $x$ in the other language.
% We use $\mbox{margin}(a, b) = a/b$ as our margin function.
